# Supplementary material for: Experimental Dispersion Relation of Surface Waves Along a Torus of Fluid
Source: arXiv:2108.08005 source file (2021-08-18)
Supplement: Supplementary file 1 [file SM.pdf]

# SUPPLEMENTAL MATERIALS
# "Experimental Dispersion Relation of Surface Waves Along a Torus of Fluid"

Filip Novkoski,[1] Eric Falcon,[1] and Chi-Tuong Pham[2]

[1] *Université de Paris, MSC, UMR 7057 CNRS, F-75 013 Paris, France*
[2] *Université Paris Saclay, LIMSI, UPR 3251 CNRS, F-91 405 Orsay, France*

In this supplemental material, we present movies (Sec. I) and images (Sec. II) of azimuthal surface waves propagating along a torus of fluid as well as additional details on the model used to describe the cutoff frequency of the sinuous mode (Sec. III). Additional dispersion relations for different torus widths are also presented (Sec. IV), followed by details on the numerical simulations used to compute the cutoff frequencies of the sloshing modes (Sec. V).

## I. MOVIES

- sweep.mp4 (20 s): Propagating azimuthal waves along a torus (sweep-sine forcing). Torus width $W = 1.6$ cm.
- torus_slim_polygon.mp4 (10 s): Standing waves on a slim torus ($W = 1.5$ cm) forced at $f = 1.9$ Hz.
- torus_wide_polygon.mp4 (10 s): Standing waves on a wide torus ($W = 3$ cm) forced at $f = 2.5$ Hz.

## II. IMAGES

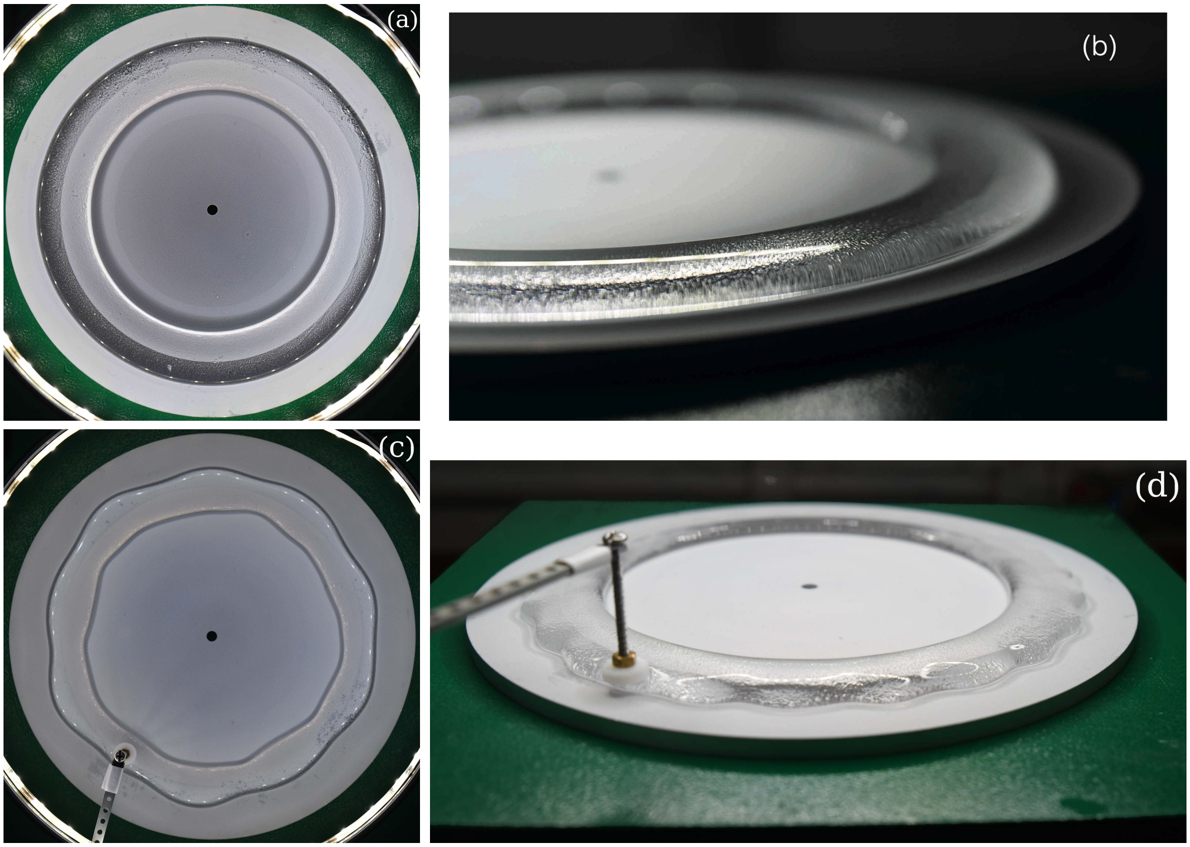


FIG. S1: Stable torus with no forcing: (a) top view and (b) side view. Torus submitted to a sinusoidal forcing: (c) $f = 2$ Hz (top view) and (d) $f = 6$ Hz (side view). Torus width $W = 2.3$ cm.

## III. SINUOUS CUTOFF FREQUENCY MODEL

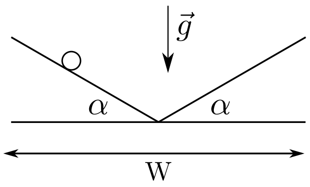


FIG. S2: A solid bead slides at the surface of a wedge-shaped substrate. The angle of the wedge with the horizontal is $\alpha$. The horizontal amplitude of the displacement is $W/2$.

We consider the situation depicted in Figure S2: a bead slides at the surface of a wedge shaped substrate, inclined by an angle $\alpha$. We will assume that the center of mass of the cross section of a torodial drop oscillates in a way similar to the bead. The Lagrangian of the problem is thus $L(y, \dot{y}) = \frac{1}{2}m(1 + \tan^2\alpha)\dot{y}^2 - mg\tan\alpha|y|$. The time $t$ it takes for the bead to slide from the top position of one slope down to the wedge bottom then reads

$$t^2 = \frac{2W}{g\sin(2\alpha)}. \tag{S1}$$

It is the quarter of the full period $T$ of the motion, which then reads $T = 4\sqrt{2W/[g\sin(2\alpha)]}$, so that the angular frequency corresponding to this oscillation is

$$\omega = \frac{2\pi}{T} = \frac{\pi}{2}\sqrt{\frac{g\sin(2\alpha)}{2W}} \tag{S2}$$

## IV. DISPERSION RELATIONS FOR DIFFERENT TORUS WIDTHS

The dispersion relations of azimuthal waves along the inner and outer borders are shown in Fig. S3 for different widths $W$. The larger $W$, the more sloshing branches are visible (their cutoff frequencies scale as $W^{-1}$). The larger $W$, the less visible the varicose branch for the inner border and the less visible the sinuous branch for the outer border.

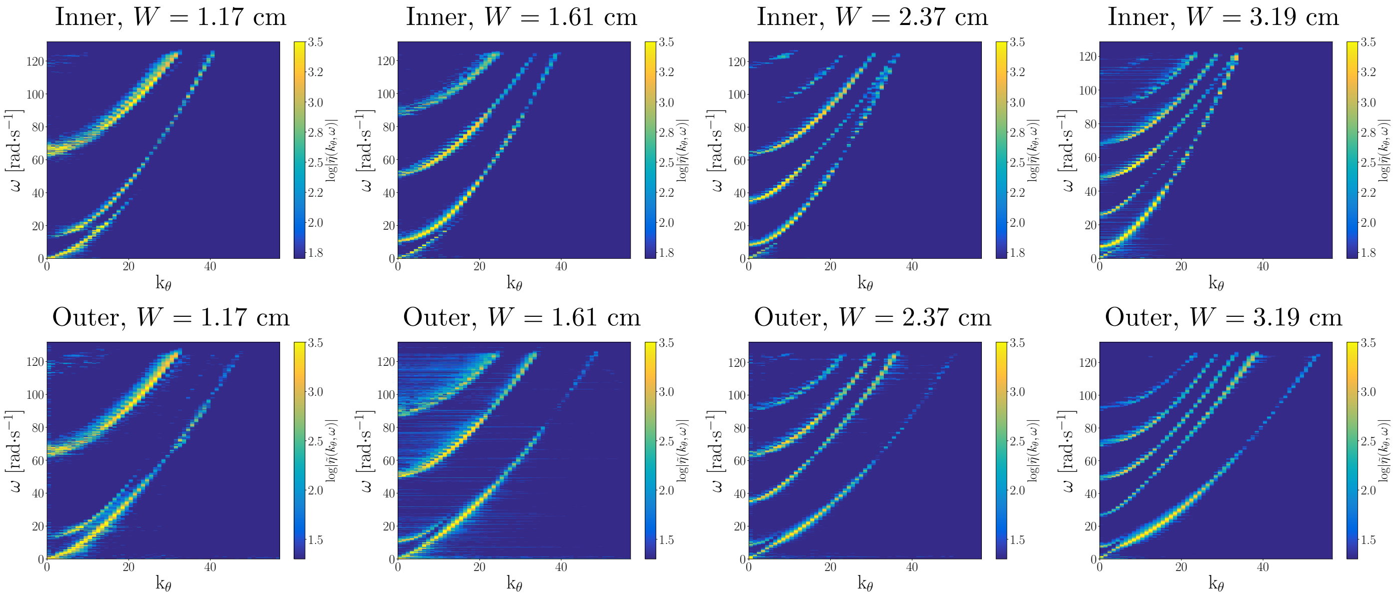


FIG. S3: Dispersion relations of azimuthal waves along the inner and borders for different torus widths $W$. The case $W = 3.19$ cm corresponds to those of Fig. 2 and 3 in the article.

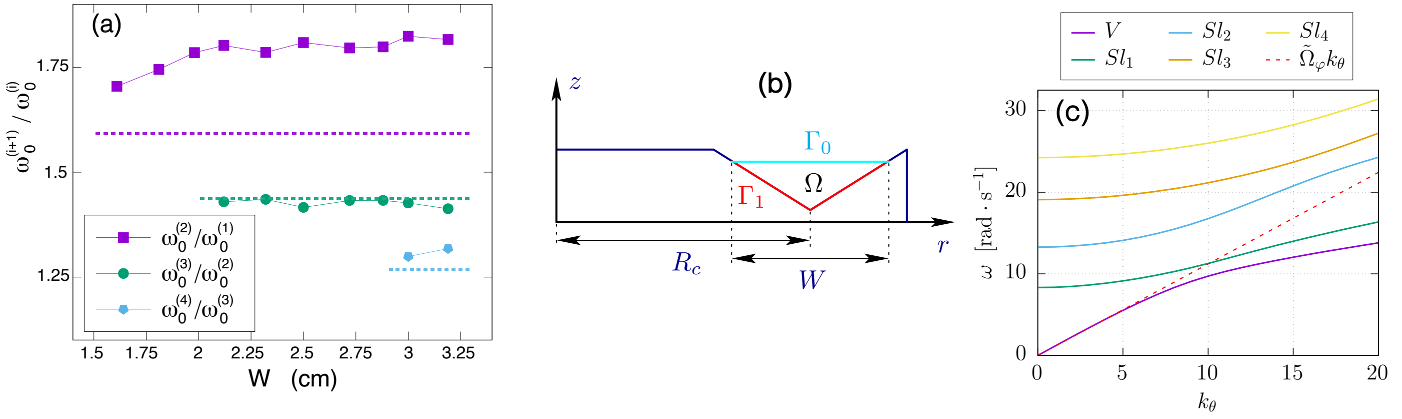


FIG. S4: (a) Sloshing cutoff frequency ratios $\omega_0^{(i+1)}/\omega_0^{(i)}$ for different torus widths $W$: experiments (symbols), and simulations $M(i+1)/M(i)$ (dashed lines). These ratios are roughly constant with $W$. $R_c = 7$ cm. (b) Notations for the numerical problem. (c) Numerical dispersion relation for a torus of radius $R_c = 7$ cm and width $W = 3.2$ cm. The varicose together with the four first sloshing branches are displayed, and lead to $M(i+1)/M(i)$ values.

## V. SLOSHING CUTOFF FREQUENCIES

As shown in the main article, the sloshing branches are well described by Eq. (5), i.e.

$$\omega_{Sl_i}^2 = \left(\omega_0^{(i)}\right)^2 + c^2 \left(\frac{k_\theta}{R_c}\right)^2 \tag{S3}$$

with $c = \sqrt{g_{\text{eff}} R_c}$ and $\omega_0^{(i)}$ the cutoff frequencies at $k_\theta = 0$. The cutoffs are found to scale as $\omega_0^{(i)} \sim W^{-1}$ (see bottom inset of Fig. 4 of the article), and are well described (see solid lines) by $\omega_0^{(i)} = M(i)\sqrt{g_{\text{eff}} R_c}/W$ with $M(i)$ a function of the index $i$ of the sloshing branche. $M(i)$ is computed numerically as explained below. The experimental cutoff ratios $\omega_0^{(i+1)}/\omega_0^{(i)}$ are then plotted in Fig. S4a and compared with numerically found values $M(i+1)/M(i) = 1.59$, 1.44 and 1.23 for $i = 1$, 2 and 3. These cutoff frequency ratios are found to be constant for $W \geq 2$ cm. Note that the departure of 20% from the experiments for $i = 1$ is due to capillary effects (capillary cap above the wedge [32]).

Details of numerical calculations of the sloshing modes are given below. They can be performed only if surface tension is neglected. Under this assumption, the free interface $\Gamma_0$ is flat, of width $W$ and its center is located at $r = R_c$ (see Fig. S4b) in cylindrical coordinates $(r, \theta, z)$. The wetted region at the wedge is denoted $\Gamma_1$. At rest, the azimuthal section of the liquid is a wedge of angle $\alpha$ with the horizontal, denoted $\Omega$. In the inviscid and irrotational case, if the velocity potential is such that

$$\Psi(r, \theta, z) = \exp[i(k_\theta \theta - \omega t)]\Phi(r, z), \tag{S4}$$

the system is governed by the following set of equations [26], in the linear limit

$$\left[\frac{\partial^2}{\partial r^2} + \frac{1}{r}\frac{\partial}{\partial r} + \frac{\partial^2}{\partial z^2}\right]\Phi - \frac{k^2}{r^2}\Phi = 0, \qquad \forall (r, z) \in \Omega \tag{S5}$$

$$\partial_n \Phi|_{\Gamma_1} = 0, \tag{S6}$$

$$\partial_n \Phi|_{\Gamma_0} = \frac{\omega^2}{g}\phi|_{\Gamma_0}. \tag{S7}$$

Equation (S5) is the incompressibility whereas Eq. (S6) reflects the imperviousness of the wedge solid surface $\Gamma_1$, and Eq. (S7) is the combination of the kinetic and Bernoulli equations at the free interface. The dispersion relation is numerically obtained from Eqs. (S5–S7) as a generalized eigenvalue problem [for a given $k_\theta$, we find a non-zero function $\Phi$ and a real $\omega$ satisfying Eqs. (S5–S7)]. The numerical dispersion relation is shown in Fig. S4c, and is close to the experimental one for sloshing modes whereas the varicose mode departs at large $k_\theta$ since surface tension is neglected. The ratios of sloshing cutoff frequencies, $M(i+1)/M(i)$, are then inferred.
